# Supplementary material for: Generative Unlearning for Any Identity
Source: arXiv:2405.09879 source file (2024-05-16)
Supplement: Supplementary file 2 [file fig_tsne_domain.tex]

\begin{figure}[!t]
    \centering
    \includegraphics[width=0.6\columnwidth]{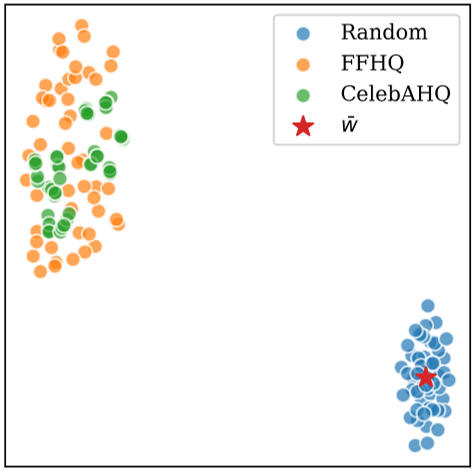}
    \caption{The distribution of identities in the latent space across three scenarios - Random (blue), In-domain (yellow), and Out-of-domain (green). We sampled 50 images per scenario.}
    \label{fig:tsne_domain}
\end{figure}
