# Supplementary material for: Generative Unlearning for Any Identity
Source: arXiv:2405.09879 source file (2024-05-16)
Supplement: Supplementary file 3 [file tab_domain_norm.tex]

\begin{table}[!t]
\centering
\resizebox{0.8\columnwidth}{!}{%
\begin{tabular}{c|cccc}
\toprule[1.1pt]
 & Random & FFHQ & CelebAHQ \\ \hline
$\Vert w_{id} \Vert_2$ & 33.12 \scriptsize{$\pm$ 2.55} & 70.92 \scriptsize{$\pm$ 2.27} & 71.14 \scriptsize{$\pm$ 1.35} \\ \bottomrule[1.1pt]
\end{tabular}%
}
\caption{Average norm of $w_{id}$ calculated in Random, FFHQ, CelebAHQ dataset.}
\vspace{-0.3cm}
\label{tab:domain_norm}
\end{table}
