# Supplementary material for: Generative Unlearning for Any Identity
Source: arXiv:2405.09879 source file (2024-05-16)
Supplement: Supplementary file 4 [file tab_std_figure_5.tex]

\begin{table}[!t]
    \centering
    \resizebox{\columnwidth}{!}{%
        \begin{tabular}{l|ccc|ccc}
        \toprule[1.1pt]
        \multirow{2}{*}{Method} &
          \multicolumn{3}{c|}{In-Domain (FFHQ)} &
          \multicolumn{3}{c}{Out-of-Domain (CelebAHQ)} \\ \cline{2-4}\cline{5-7}
         &
          ID  &
          FID\textsubscript{pre} &
          $\Delta$FID\textsubscript{real} &
          ID&
          FID\textsubscript{pre} &
          $\Delta$FID\textsubscript{real}\\ \hline
          Baseline & \scriptsize{$\pm$ 0.07} & \scriptsize{$\pm$ 1.04} & \scriptsize{$\pm$ 0.77}
                   & \scriptsize{$\pm$ 0.07} & \scriptsize{$\pm$ 0.88} & \scriptsize{$\pm$ 0.83} 
                   \\
        \textbf{Ours} & \scriptsize{$\pm$ 0.08} & \scriptsize{$\pm$ 0.13} & \scriptsize{$\pm$ 0.15} 
                   & \scriptsize{$\pm$ 0.08} & \scriptsize{$\pm$ 0.24} &  \scriptsize{$\pm$ 0.20} \\ \bottomrule[1.1pt]
        \end{tabular}%
    }
    \caption{Standard deviations corresponding to the results of Table 5 in the main paper.}
\label{tab:std_figure_5}
\end{table}
